# Supplementary material for: Field-based Design of a Resonant Dielectric Antenna for Coherent Spin-Photon Interfaces
Source: arXiv:2101.02366 ancillary file (2021-01-07)
Supplement: Supplementary file 1 [file SI.pdf]

# Field-based design of a resonant dielectric antenna for coherent spin-photon interfaces: supplemental document

This document provides supplementary information for "Field-based design of a resonant dielectric antenna for coherent spin-photon interfaces." We present the transition from far field to near field and illustrate the transfer matrix model for estimating the near field of the dielectric perturbation. We also show the optimization process such as curving the mirror to better match the phase front of the dipole source. Finally, we provide the antenna parameters of our final designs.

## 1. TRANSITION FROM FAR FIELD TO NEAR FIELD

We calculate the far-field distribution for a given near-field distribution $\vec{H}(x,y)$ and $\vec{E}(x,y)$ on the surface $S$ (Fig. S1). In the color plot of fig. S1(b-g), we normalized all the field component distributions by their maximum absolute value.

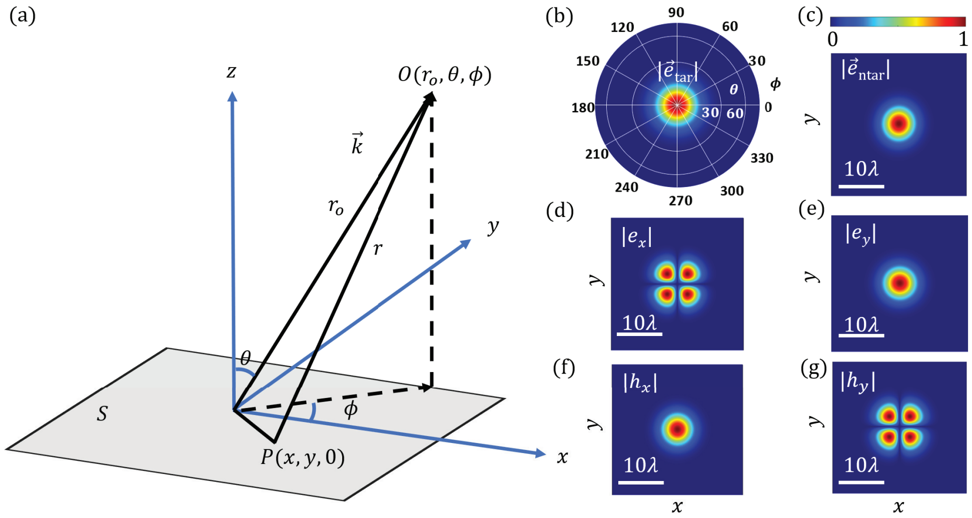


**Fig. S1.** (a) The near field at the point $P(x,y,0)$ on the surface $S$ and far field at the point $O(r_o,\theta,\phi)$. (b) Normalized target far field $|\vec{e}_{\text{tar}}| = |\vec{E}_{\text{tar}}(\theta,\phi)|/\max(|\vec{E}_{\text{tar}}(\theta,\phi)|)$. (c-g) Normalized target near field $|\vec{e}_{\text{ntar}}| = |\vec{E}_{\text{ntar}}(x,y)|/\max(|\vec{E}_{\text{ntar}}(x,y)|)$, target electric near-field $x$-component $|e_x| = |E_x(x,y)|/\max(|E_x(x,y)|)$, target electric near-field $y$-component $|e_y| = |E_y(x,y)|/\max(|E_y(x,y)|)$, target magnetic near-field $x$-component $|h_x| = |H_x(x,y)|/\max(|H_x(x,y)|)$, and target magnetic near-field $y$-component $|h_y| = |H_y(x,y)|/\max(|H_y(x,y)|)$, respectively.

The equivalent sources in the plane $S$ can be expressed with the surface electric current $\vec{J}_s = \vec{n}\times\vec{H} = -\vec{x}H_y + \vec{y}H_x$ and surface magnetic current $\vec{M}_s = -\vec{n}\times\vec{E} = \vec{x}E_y - \vec{y}E_x$ [1]. Here $\vec{n} = \vec{z}$ are unit vectors that are perpendicular to the surface. $\vec{E}$ and $\vec{H} = \vec{B}/\mu_0$ are the electric and magnetic fields, respectively. The 2D Fourier transformation $(FT_2)$ of the field $f(x,y)$ is

$$FT_2(f(x,y)) = \int\int \mathrm{d}x\mathrm{d}y f(x,y)e^{(ik_x x + k_y y)}, \tag{S1}$$

where $k_x = k\sin\theta\cos\phi, k_y = k\sin\theta\sin\phi$, $k = \frac{2\pi}{\lambda}$, and $\lambda$ is the free space wavelength. The radiation vectors $\vec{N}$ and $\vec{L}$ are expressed with the 2D Fourier transform of the surface current $\vec{J}_s$

and $\vec{M}_s$ ,

$$\vec{N} = \int_S \vec{J}_s e^{i(k_x x + k_y y)} \mathrm{d}S = FT_2(\vec{J}_s), \tag{S2}$$

$$\vec{L} = \int_S \vec{M}_s e^{i(k_x x + k_y y)} \mathrm{d}S = FT_2(\vec{M}_s). \tag{S3}$$

Here $(x, y, 0)$ are the coordinates of the point $P$ in the plane $S$. In homogeneous isotropic media, the retarded potential $\vec{A}$ and the second retarded potential $\vec{F}$ are

$$\vec{A} = \mu_0 \int_S \frac{\vec{J}_s e^{-ikr}}{4\pi r} \mathrm{d}S = \mu_0 \frac{-e^{ikr_o}}{4\pi r_o} \vec{N}, \tag{S4}$$

$$\vec{F} = \varepsilon_0 \int_S \frac{\vec{M}_s e^{-ikr}}{4\pi r} \mathrm{d}S = \varepsilon_0 \frac{-e^{ikr_o}}{4\pi r_o} \vec{L}, \tag{S5}$$

where $r$ is the distance between the surface element $\mathrm{d}S$ and the point $O$, and $r_o$ is the distance between the origin $(0, 0, 0)$ and the point $O$. The derivation here follows that in the reference [1].

The monochromatic far field can be expressed in terms of retarded potentials as $\vec{E} = -i\omega\vec{A} - \frac{i\omega}{k^2}\nabla(\nabla \cdot \vec{A}) - \frac{1}{\varepsilon_0}\nabla \times \vec{F}$, $\vec{H} = -i\omega\vec{F} - \frac{i\omega}{k^2}\nabla(\nabla \cdot \vec{F}) - \frac{1}{\mu_0}\nabla \times \vec{A}$. Here $\omega$ is the angular frequency, $\varepsilon_0$ is the permittivity of vacuum, and $\mu_0$ is the magnetic permeability in vacuum. Under the assumption that all terms in the fields decaying faster than $1/r_o$ can be neglected, the electric field components at an arbitrary point $O$ are $E_\theta = \eta H_\phi = -i\frac{e^{-ikr_o}}{2\lambda r_o}(\eta N_\theta + L_\phi)$ and $E_\phi = -\eta H_\theta = i\frac{e^{-ikr_o}}{2\lambda r_o}(-\eta N_\phi + L_\theta)$, where $\eta = \sqrt{\frac{\mu_0}{\varepsilon_0}}$ and $(r_o, \theta, \phi)$ represent the coordinates of the point $O$ in spherical coordinates. The $\theta$ and $\phi$ components of the radiation vector $\vec{N}$ and $\vec{L}$ are

$$N_\theta = (N_x \cos\phi + N_y \sin\phi)\cos\theta = -FT_2(H_\perp)\cos\theta, \tag{S6}$$

$$N_\phi = -N_x \sin\phi + N_y \cos\phi = FT_2(H_\parallel), \tag{S7}$$

$$L_\theta = (L_x \cos\phi + L_y \sin\phi)\cos\theta = FT_2(E_\perp)\cos\theta, \tag{S8}$$

$$L_\phi = (-L_x \cos\phi + L_y \sin\phi) = -FT_2(E_\parallel), \tag{S9}$$

where $N_x = -FT_2(H_y)$, $N_y = FT_2(H_x)$, $L_x = FT_2(E_y)$, and $L_y = -FT_2(E_x)$ . The field relations are

$$E_\parallel = E_x \cos\phi + E_y \sin\phi, \tag{S10}$$

$$H_\parallel = H_x \cos\phi + H_y \sin\phi, \tag{S11}$$

$$E_\perp = -E_x \sin\phi + E_y \cos\phi, \tag{S12}$$

$$H_\perp = -H_x \sin\phi + H_y \cos\phi. \tag{S13}$$

Thus, we can find the relations

$$\eta N_\theta + L_\phi = -FT_2(\eta H_\perp)\cos\theta - FT_2(E_\parallel), \tag{S14}$$

$$-\eta N_\phi + L_\theta = -FT_2(\eta H_\parallel) - FT_2(E_\perp)\cos\theta. \tag{S15}$$

For a plane wave propagating with polar angle $\theta$, it follows that $\eta H_\perp \cos\theta = E_\parallel$ and $\eta H_\parallel = -E_\perp \cos\theta$. Then we have

$$FT_2(\eta H_x) = FT_2(\eta H_\parallel)\cos\phi - FT_2(\eta H_\perp)\sin\phi, \tag{S16}$$

$$FT_2(\eta H_y) = FT_2(\eta H_\parallel)\sin\phi + FT_2(\eta H_\perp)\cos\phi, \tag{S17}$$

$$FT_2(E_x) = FT_2(E_\parallel)\cos\phi - FT_2(E_\perp)\sin\phi, \tag{S18}$$

$$FT_2(E_y) = FT_2(E_\parallel)\sin\phi + FT_2(E_\perp)\cos\phi. \tag{S19}$$

We can recover $H_x$, $H_y$, $E_x$, and $E_y$ once we know the target near field $E_\theta$ and $E_\phi$ using the following equations:

$$FT_2(\eta H_x) = FT_2(\eta H_\parallel)\cos\phi - FT_2(\eta H_\perp)\sin\phi = -i\lambda r_o e^{ikr_o}(-E_\phi \cos\phi - E_\theta \sin\phi/\cos\theta), \tag{S20}$$

$$FT_2(\eta H_y) = FT_2(\eta H_{\|}) \sin\phi + FT_2(\eta H_{\perp}) \cos\phi = -i\lambda r_o e^{ikr_o}(-E_\phi \sin\phi + E_\theta \cos\phi / \cos\theta), \quad \text{(S21)}$$

$$FT_2(E_x) = FT_2(E_{\|}) \cos\phi - FT_2(E_{\perp}) \sin\phi = -i\lambda r_o e^{ikr_o}(E_\theta \cos\phi - E_\phi \sin\phi / \cos\theta), \quad \text{(S22)}$$

$$FT_2(E_y) = FT_2(E_{\|}) \sin\phi + FT_2(E_{\perp}) \cos\phi = -i\lambda r_o e^{ikr_o}(E_\theta \sin\phi + E_\phi \cos\phi / \cos\theta). \quad \text{(S23)}$$

For a target far field $\vec{E}_{\text{tar}}(\theta,\phi) = E_r(\theta,\phi)\vec{r} + E_\theta(\theta,\phi)\vec{\theta} + E_\phi(\theta,\phi)\vec{\phi}$ in polar coordinates, we can obtain the target near field $H_\perp, E_\perp, H_\|$ and $E_\|$ using the inverse Fourier transform and then obtain $H_x, H_y, E_x$, and $E_y$ as the target near field. For a target polarized paraxial Gaussian field $\vec{E}_{\text{tar}}(\theta,\phi) = E_0 \exp(-\tan^2\theta/0.4^2)\vec{y} = E_0 \exp(-\tan^2\theta/0.4^2) \times (\sin\theta \sin\phi\, \vec{r} + \cos\theta \sin\phi\, \vec{\theta} + \cos\phi\, \vec{\phi})$, we have

$$E_r(\theta,\phi) = \eta H_\phi(\theta,\phi) = E_0 \sin\theta \sin\phi \cdot \exp(-\tan^2\theta/0.4^2), \quad \text{(S24)}$$

$$E_\theta(\theta,\phi) = \eta H_\phi(\theta,\phi) = E_0 \cos\theta \sin\phi \cdot \exp(-\tan^2\theta/0.4^2), \quad \text{(S25)}$$

$$E_\phi(\theta,\phi) = -\eta H_\theta(\theta,\phi) = E_0 \cos\phi \cdot \exp(-\tan^2\theta/0.4^2), \quad \text{(S26)}$$

where $E_0$ is the target field amplitude. We show an example of such a target far field $\vec{E}_{\text{tar}}(\theta,\phi)$ to calculate the related target near field $\vec{E}_{\text{ntar}}(x,y)$ with $x$ and $y$ components in fig. S1(b-g).

We notice that $\max(|E_y(x,y)|)/\max(|E_x(x,y)|) = 190$ in the calculation. As a result, $|E_y(x,y)|$ and $|H_x(x,y)|$ will be the primary components in the target near field for such a target far field $\vec{E}_{\text{tar}}(\theta,\phi) = E_0 \exp(-\tan^2\theta/0.4^2)\vec{y}$.

## 2. TRANSFER MATRIX MODEL

To test the mode overlap between the antenna far field and target far field, we need to do 3D FDTD simulations as shown in the main text. When the target far field has a Gaussian distribution and is polarized in the $y$ direction, we know the target near field will have the primary electric field component of $E_y$ and the primary magnetic field component of $H_x$ with circular symmetric amplitude. As a result, we can simplify the model using 2D FDTD simulation in $x$-$z$ plane and attempt to match the near field along the $x$-axis, $\vec{E}_{\text{ntar}}(x,z_0) = E_y(x,z_0)\vec{y}$, where $z_0$ is the near field monitor $z$ coordinate. Then, we can match the far-field distribution of $\vec{E}_{\text{tar}}(\theta,0)$. Here, we use a transfer matrix model (TMM) to predict the antenna near field. The TMM uses a scalar approximation (the electric field only has a $y$ component) and single-mode approximation, (the field distribution immediately after transmission or reflection is identical to the incident slab mode distribution). The TMM provides a good initial design to increase the mode overlap between the antenna near field and target near field in 3D FDTD simulations [2]. The recipe for using the transfer matrix model to predict the antenna near field with slot scattering layers is:

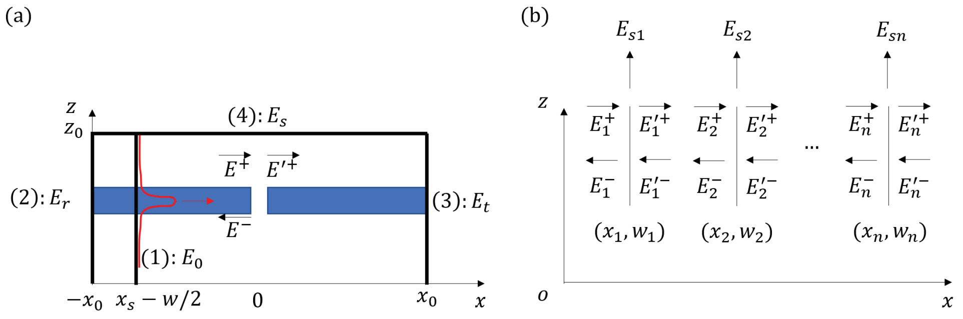


**Fig. S2.** (a) The single-slot model setting in the $x$-$z$ cross-section. The center of a diamond slab with $H = 150$ nm thickness is located at $z = 0$ $\mu$m. The center of the air slot with width $w$ is located at $x = 0$ $\mu$m in the slab. The slab mode complex input field amplitude $E^+$ is recorded at (1), the complex reflected field amplitude $E^-$ at (2), the complex transmitted field amplitude $E'^+$ at (3), and the complex scattered field amplitude $E_s$ at (4). (b) The multi-slot model showing the effect of cascading many slots. The $i^{\text{th}}$ slot with width $w_i$ and location $x_i$ will have complex input and output fields amplitude from the left $(E_i^+, E_i^-)$ and right sides $(E_i'^+, E_i'^-)$ in the slab. Every slot $(i = 1, 2, ...)$ has the complex scattering near fields amplitude $E_{si}(x - x_i, z_0, w_i)$.

1. Calculate the fundamental TE slab ($y$-polarized) mode propagating in $+x$ direction to know the effective wave vector $k_{\text{eff}}$ without a slot. The slab should be thin enough to support only a single mode in the $z$ direction.

2. Calculate the transmission coefficient $t(w)$ and reflection coefficient $r(w)$ of different slot widths $w$.

3. Calculate the scattering near field for a single slot, which has a center located at $x = 0$ $\mu$m. Repeat the calculation with different slot widths $w$, and to obtain a lookup table of scattering near fields $E_s(x, z_0, w)$, $H_s(x, z_0, w)$ for different slot widths $w$.

4. For a slot array design with $n$ slots, each slot has a location $x_i$ and width $w_i$ $(i = 1, 2, ..., n)$. We can obtain the transfer matrix $T_i$ [defined in Eq. S29] from $x_i$ and $w_i$ that connects the fields' $y$-component on either side of the slot $(E_i^+, E_i^-, E_i'^+$, and $E_i'^-)$ as illustrated in fig. S2(a). The propagation of the slab mode between neighboring slots $i$ and $i+1$ is described by the propagation matrix $\Theta_i$, which is defined in Eq. S30.

5. By coherently adding the scattered fields from all the slots, we obtain the antenna near-field distribution $\vec{E}_{\text{near}}(x, z_0)$.

Let us consider each step in the recipe in more details: In step 1, we determine the fundamental TE slab mode $E_0(x_s - w/2, z)\vec{y}$ at monitor (1) without a slot as illustrated in fig. S2(a). The slab mode is given by $E(x, z)\vec{y} = E_0 \exp(ik_{\text{eff}}x) f(z)\vec{y}$, where $f(z)$ is a dimensionless field distribution along the $z$ direction. For a slot width $w$ in step 2, we obtain the complex input field amplitude $E^+ = E_0 \exp[ik_{\text{eff}}(-x_s)]$ using the parameters in step 1. The complex reflection field amplitude is $E^- = E_r \exp[ik_{\text{eff}}(x_0 - w/2)]$ using the data at monitor (2). The complex transmission field amplitude is $E'^+ = E_t \exp[-ik_{\text{eff}}\,(x_0 - w/2)]$ using the data at monitor (3). Then, we calculate the transmission coefficient $t(w) = E'^+/E^+$ and the reflection coefficient $r(w) = E^-/E^+$.

In step 3, we obtain $E_s(x, z_0)\vec{y}$ from the near-field monitor (4) when the input field is propagating from left to right. The location of the source in the FDTD simulation is adjusted for each slot width such that $E^+(-w/2, 0)\vec{y}$ is the same in all the simulations. We note that the scattering near field is asymmetric and is thus given by $E_s(-x, z_0)\vec{y}$ for an input propagating from right to left.

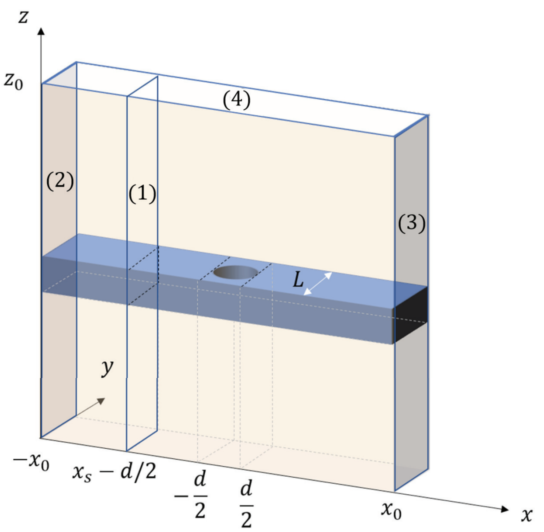


**Fig. S3.** Simulation setting for the holes model. The center of a diamond slab with $H = 150$ nm thickness is located at $z = 0$ $\mu$m. The center of the air holes with diameter $d$ is located at $x = 0$ $\mu$m in the slab. A periodic condition exists in $y$ direction with the periodic length $L$. Here, four monitors ((1), (2), (3), (4)) record the fundamental TE slab mode input, reflection, transmission, and scattering near field, respectively.

In step 4, we build the equation for linking the input and output field $y$-component from the left side $(E_i^+, E_i^-)$ and right side $(E_i'^+, E_i'^-)$ for the $i^{\text{th}}$ slot in the slab. Since the transmission coefficient and reflection coefficient will remain the same when considering the left to right transmission and right to left transmission, the equations are

$$E_i'^{+} = t(w_i)E_i^{+} + r(w_i)E_i'^{-}, \tag{S27}$$

$$E_i^{-} = r(w_i)E_i^{+} + t(w_i)E_i'^{-}, \tag{S28}$$

$$\begin{bmatrix} E_i^{+} \\ E_i^{-} \end{bmatrix} = T_i \begin{bmatrix} E_i'^{+} \\ E_i'^{-} \end{bmatrix} = \begin{bmatrix} \frac{1}{t(w_i)} & -\frac{r(w_i)}{t(w_i)} \\ \frac{r(w_i)}{t(w_i)} & \frac{t(w_i)^2 - r(w_i)^2}{t(w_i)} \end{bmatrix} \begin{bmatrix} E_i'^{+} \\ E_i'^{-} \end{bmatrix}, \tag{S29}$$

$$\begin{bmatrix} E_i'^{+} \\ E_i'^{-} \end{bmatrix} = \Theta_i \begin{bmatrix} E_{i+1}^{+} \\ E_{i+1}^{-} \end{bmatrix} = \begin{bmatrix} \exp(-ik_{\text{eff}}(x_{i+1} - x_i)) & 0 \\ 0 & \exp(ik_{\text{eff}}(x_{i+1} - x_i)) \end{bmatrix} \begin{bmatrix} E_{i+1}^{+} \\ E_{i+1}^{-} \end{bmatrix}. \tag{S30}$$

Here, we have a boundary condition at the $n^{\text{th}}$ slot that $E_n'^{-} = 0$ indicating there is no source input outside the slab. Then we can express all the fields in terms of $E_n'^{+}$.

In step 5, the contribution to the near field from the $i^{\text{th}}$ slot will be $E_{si} = (E_i^{+}/E_n'^{+})E_s(x - x_i, z_0) + (E_i^{+}/E_n'^{+})E_s(-x - x_i, z_0)$. The total contribution from all the slots to the near field can be written as

$$\vec{E}_{\text{near}}(x, z_0) = \sum_{i=1}^{n} E_{si}\vec{y}. \tag{S31}$$

For a design using holes rather than slots, a similar TMM recipe is used. The $i^{\text{th}}$ layer of holes is placed at $x_i$, with hole diameter $d_i$ and separation $L_i (i = 1, 2, ..., n)$. The hole separation $L$ will be the same as the periodic length in the $y$ direction of the 3D FDTD simulation illustrated in fig. S3. Here, we define the hole diameter-to-distance ratio $p = d/L$. As with the slots, we use FDTD simulations with a single scatter layer to obtain a lookup table of the transmission coefficient $t(d, p)$, the reflection coefficient $r(d, p)$, and the scattering near field $y$-component $E_s(x, z_0), H_s(x, z_0)$ for different values of the parameters $d$ and $p$. Since the slot design lookup table will only relate to the slot width $w$, the holes design has an additional degree of freedom to tune the results.

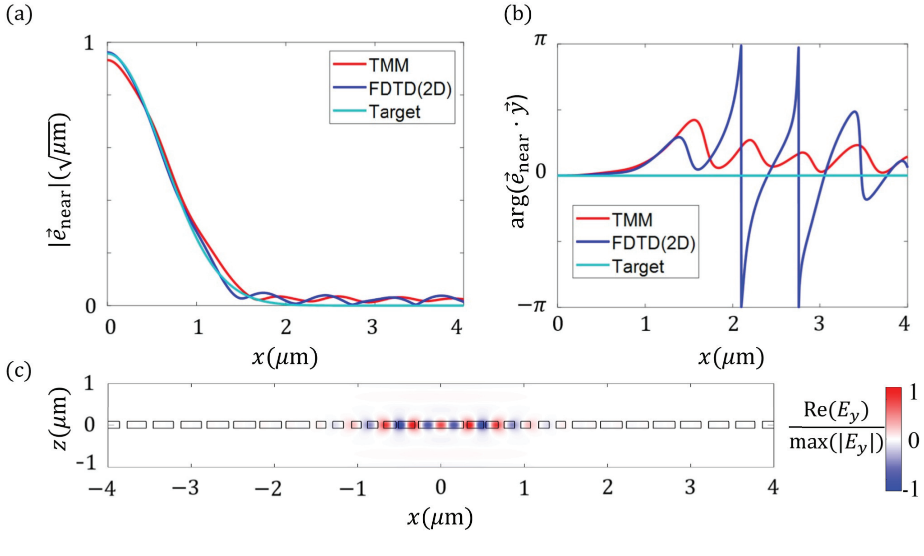


**Fig. S4.** (a) Comparison between the normalized target near field $|\vec{e}_{\text{ntar}}|$ (cyan) and the normalized near field $|\vec{e}_{\text{near}}|$ calculated using the TMM (red) or a 2D FDTD simulation (blue). (b) Plots of the phase, $\arg(\vec{e}_{\text{near}} \cdot \vec{y})$, of each field in (a). (c) The $x$-$z$ cross-section of the diamond slab with the normalized electric field $\text{Re}(E_y(x,z))/\max(|E_y(x,z)|)$ overlaid; the green line shows the edge of the dielectric material.

In the TMM, we calculate the power transmitted in both the $x$ and $z$ direction

$$P_z = \int_{-x_0}^{x_0} [\text{Re}[E_x(x, z_0)H_y^*(x, z_0) - E_y(x, z_0)H_x^*(x, z_0)]\text{d}x, \tag{S32}$$

$$P_x = \int_{-z_0}^{z_0} [\text{Re}[E_y(x,z_0)H_z^*(x,z_0) - E_z(x,z_0)H_y^*(x,z_0)]\text{d}z. \tag{S33}$$

As a result, we know $P_z$ and $P_x$ in the TMM and calculate the $z$ direction power ratio,

$$T_z = \frac{P_z}{P_x + P_z}. \tag{S34}$$

The 1D mode overlap $\kappa_{1\text{D}}$ between the antenna near field $\vec{E}_{\text{near}}(x)$ and the target near field $\vec{E}_{\text{ntar}}(x)$ is

$$\kappa_{1\text{D}} = |\int_{-x_0}^{x_0} \vec{e}_{\text{near}} \cdot \vec{e}^{\,*}_{\text{ntar}} \text{d}x|, \tag{S35}$$

where $\vec{e}_{\text{near}}$ is the normalized antenna near field that satisfies $\int_{-x_0}^{x_0} |\vec{e}_{\text{near}}|^2 \text{d}x = T_z$. $\vec{e}_{\text{near}} = C_{\text{near}}\vec{E}_{\text{near}}(x)$, where $C_{\text{near}}$ is a normalization factor. $\vec{e}_{\text{ntar}}$ is the normalized target near field that satisfies $\int_{-x_0}^{x_0} |\vec{e}_{\text{ntar}}|^2 \text{d}x = 1$. $\vec{e}_{\text{ntar}} = C_{\text{ntar}}\vec{E}_{\text{ntar}}(x)$, where $C_{\text{ntar}}$ is a normalization factor. Figure S4 shows a comparison between the antenna near field $\vec{e}_{\text{near}}$ calculated with both the TMM and a 2D FDTD simulation. The overlap $\kappa_{1D}$ is 99.2% using the TMM with the antenna structure in fig. S4(c), while $\kappa_{1\text{D}} = 99.0\%$ using the 2D FDTD simulation. Though the phase, $\arg(\vec{e}_{\text{near}} \cdot \vec{y})$, is not matching well for $x > 1.5\ \mu$m, the overlap remains large since the amplitude is small in that region.

## 3. MIRROR CURVING

We start with a $y$-polarized dipole in an unpatterned slab and obtain the electric field distribution $E_y(x,y)\vec{y}$. Then, we add dielectric perturbations that follow the phase fronts of the dipole

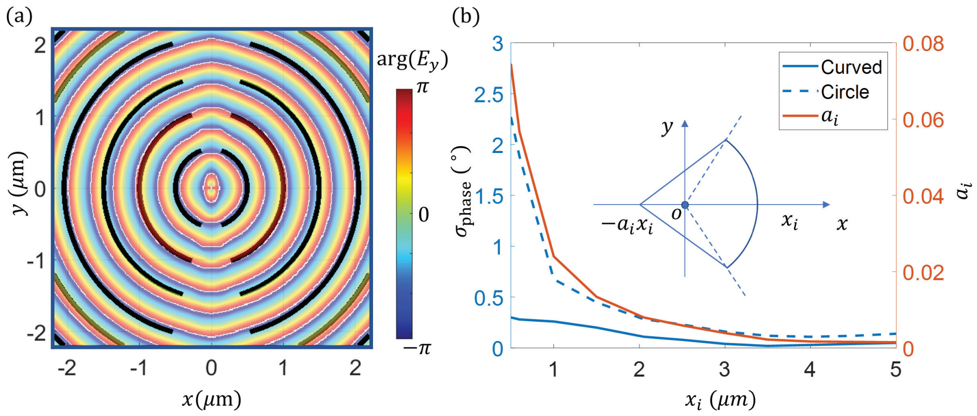


**Fig. S5.** (a) $\arg(E_y(x,y))$ distribution and the same phase front perturbation layer predicted with the curved model. (b) The $\sigma_{\text{phase}}$ of the perturbation layer at different $x_i$ predicted by the curved model (solid blue line with left $y$-axis), the $\sigma_{\text{phase}}$ of the circle model at different $x_i$ (dashed blue line with left $y$-axis), the fitting of $a_i$ with different $x_i$ (solid red line with right $y$-axis). The inset shows the use of the arc whose center is not at origin to fit the same phase front region.

field $\arg(E_y(x,y))$ as illustrated in fig. S5(a). Thus the mode will normally incident on each perturbation layer. Here, we apply the curved model to fit the phase front by using an arc whose center is not at the origin as shown in the inset of fig. S5(b). The center of the arc is located at $(x,y) = (-a_i x_i, 0)$ and the arc radius is $(1+a_i)x_i$, where $a_i$ is the fitting curvature for the perturbation layer located at $x = x_i$. We use the standard deviation $\sigma_{\text{phase}} = \sqrt{\frac{1}{N}\sum_{j=1}^{N}(\phi_j - \bar{\phi})^2}$ to evaluate the error of the same phase front region fitting curvature $a_i$ in fig. S5(b), where $\bar{\phi} = \frac{1}{N}\sum_{j=1}^{N}\phi_j$ and $\phi_j = \arg(E_y(x_j,y_j))$ is the phase at the discrete sampling points $(x_j,y_j)$ on the fitting arc $(j = 1,...,N)$. The fitting parameter $a_i$ is the optimized curvature by minimizing $\sigma_{\text{phase}}$ for the perturbation layer located at $x = x_i$. Compared with the simple circle model where the center of the arc is located at the origin $(0,0)$, the curved model has several times smaller $\sigma_{\text{phase}}$. The $\sigma_{\text{phase}}$ will be larger for the perturbation layer closer to the dipole source. But using the

curved model, the $\sigma_{\text{phase}}$ at $x_i = 0.5\ \mu$m can be 0.3°, which means only 0.5 nm standard deviation for the same phase location with a 637 nm dipole source wavelength. The curved model is ten times better than the simple circle model when $x_i < 0.5\ \mu$m. The curvature of the perturbation layer can be easily changed with a different $a_i$ for various locations $x_i$. It will also be easy to place the holes array with the same separation of holes on the arc, which is considered as the same phase front region with negligible $\sigma_{\text{phase}}$.

## 4. ANTENNA DESIGN FOR GAAS QUANTUM DOT

Besides designing the antenna for diamond color centers, we can also start the antenna design with other dielectric membranes. Here, we show the simulation results for the antenna design for a GaAs quantum dot as shown in fig. S6. Bullseye antennas have been fabricated for GaAs quantum dot in the GaAs membrane with a SiO2/Au bottom reflection layer [3]. A collection efficiency of 90% was obtained within a NA = 0.65 and a Purcell factor of 20 in the GaAs antenna design. In our design, we achieve a Purcell Factor of 316 while the mode overlap with the NA = 0.4 Gaussian far field mode is 93%, corresponding to the 87% spin-photon interface efficiency $\eta$. The detailed parameters for the antenna are shown in Table S3. The resonant wavelength can be tuned by scaling all the dimensions of the antenna structure as shown in fig. S6(c). This can be used for designing different antenna structures for the quantum dots with various wavelengths. The direct scaling will not reduce $\eta$ more than 15%. We can redo the optimization to make the efficiency higher for a specific quantum dot wavelength.

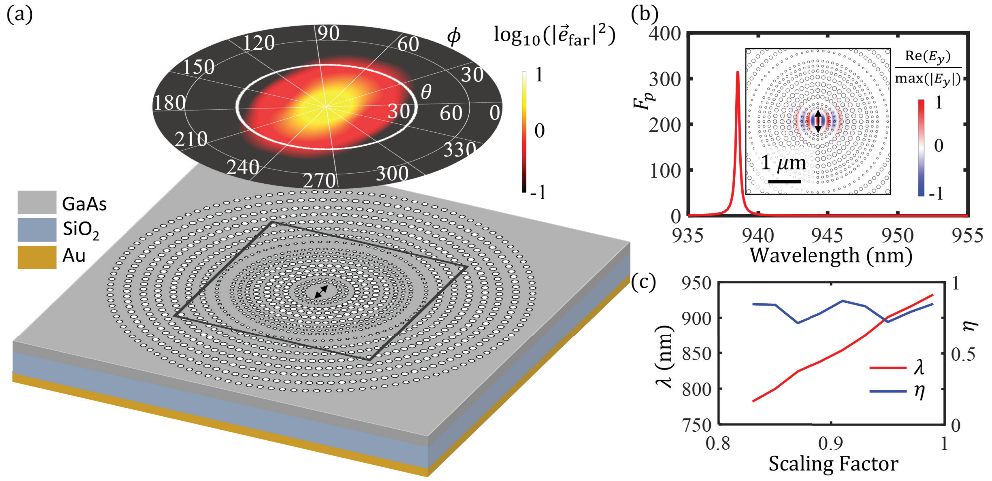


**Fig. S6.** (a) Illustration of the GaAs dielectric antenna structure, along with a plot of $\log_{10}(|\vec{e}_{\text{far}}|^2)$ showing the far-field distribution. (b) Purcell Factor spectrum of the antenna structure. The inset is a linear-scale plot of $\text{Re}(E_y)/\max(|E_y|)$ corresponding to the black square region in (a). (c) The antenna resonance frequency $\lambda$ and efficiency $\eta$ as a function of the changes in scaling factor of the whole antenna structure.

## 5. SIMULATION PARAMETERS AND OPTIMIZATION

The optimization is done using the commercially available software Lumerical with a user-defined gradient descent algorithm. The optimized parameters for the antenna structure in the main text are given in Table S1 and Table S2. In the parameter table, $a_1$ is the fitting curvature of the first perturbation layer closest to the central dipole source and $a_2$ is the fitting curvature of the next perturbation layer. The following perturbation layer curvatures $a(x)$ are determined by their locations $a(x) = \frac{a_2 x_2}{x}$. For the holey antenna, $4N$ is the number of holes in each perturbation layer.

## REFERENCES


1. J. Vuckovic, M. Loncar, H. Mabuchi, and A. Scherer, "Optimization of the q factor in photonic crystal microcavities," IEEE J. Quantum Electron. **38**, 850–856 (2002).

**Table S1. Diamond slot antenna design.** ($F_p = 154$, $\eta_2 = 0.90 \rightarrow \eta_{NV} = 0.74$ ; $\eta_{SnV} = 0.89$)

| Global | | Slot Location | | Slot Width | |
|---|---|---|---|---|---|
| $x_0$ | 5 $\mu$m | $x_1$ | 0.369 $\mu$m | $w_1$ | 41 nm |
| $y_0$ | 5 $\mu$m | $x_2$ | 0.560 $\mu$m | $w_2$ | 41 nm |
| $H$ | 150 nm | $x_3$ | 0.771 $\mu$m | $w_3$ | 66 nm |
| $z_0$ | 1 $\mu$m | $x_4$ | 0.993 $\mu$m | $w_4$ | 89 nm |
| $z_{\min}$ | 330 nm | $x_5$ | 1.204 $\mu$m | $w_5$ | 92 nm |
| $a_1$ | 1.12 | $x_6$ | 1.439 $\mu$m | $w_6$ | 96 nm |
| $a_2$ | 1.08 | $x_7$ | 1.640 $\mu$m | $w_7$ | 58 nm |
| theta | 75° | $x_8$ | 1.808 $\mu$m | $w_8$ | 50 nm |
| | | $x_9$ | 1.975 $\mu$m | $w_9$ | 55 nm |
| | | $x_{10}$ | 2.312 $\mu$m | $w_{10}$ | 48 nm |
| | | $x_{11}$ | 2.631 $\mu$m | $w_{11}$ | 58 nm |
| | | $x_{12}$ | 2.939 $\mu$m | $w_{12}$ | 60 nm |
| | | $x_{13}$ | 3.268 $\mu$m | $w_{13}$ | 90 nm |
| | | $x_{14}$ | 3.611 $\mu$m | $w_{14}$ | 73 nm |
| | | $x_{15}$ | 3.928 $\mu$m | $w_{15}$ | 93 nm |
| | | $x_{16}$ | 4.294 $\mu$m | $w_{16}$ | 111 nm |
| | | $x_{17}$ | 4.663 $\mu$m | $w_{17}$ | 120 nm |

**Table S2. Diamond holey antenna design.** ($F_p = 420$, $\eta_2 = 0.87 \rightarrow \eta_{NV} = 0.81$ ; $\eta_{SnV} = 0.86$)

| Global | | Holes Location | | Holes Diameter | | $N$ | |
|---|---|---|---|---|---|---|---|
| $x_0$ | 5 $\mu$m | $x_1$ | 0.392 $\mu$m | $d_1$ | 70 nm | $n_1$ | 5 |
| $y_0$ | 5 $\mu$m | $x_2$ | 0.564 $\mu$m | $d_2$ | 80 nm | $n_2$ | 6 |
| $H$ | 150 nm | $x_3$ | 0.776 $\mu$m | $d_3$ | 110 nm | $n_3$ | 8 |
| $z_0$ | 1 $\mu$m | $x_4$ | 0.999 $\mu$m | $d_4$ | 160 nm | $n_4$ | 8 |
| $z_{\min}$ | 335 nm | $x_5$ | 1.211 $\mu$m | $d_5$ | 150 nm | $n_5$ | 10 |
| $a_1$ | 1.16 | $x_6$ | 1.448 $\mu$m | $d_6$ | 140 nm | $n_6$ | 12 |
| $a_2$ | 1.08 | $x_7$ | 1.650 $\mu$m | $d_7$ | 100 nm | $n_7$ | 17 |
| theta | 90° | $x_8$ | 1.819 $\mu$m | $d_8$ | 80 nm | $n_8$ | 18 |
| | | $x_9$ | 1.988 $\mu$m | $w_9$ | 80 nm | $n_9$ | 19 |
| | | $x_{10}$ | 2.327 $\mu$m | $d_{10}$ | 70 nm | $n_{10}$ | 20 |
| | | $x_{11}$ | 2.647 $\mu$m | $d_{11}$ | 130 nm | $n_{11}$ | 22 |
| | | $x_{12}$ | 2.958 $\mu$m | $d_{12}$ | 140 nm | $n_{12}$ | 23 |
| | | $x_{13}$ | 3.289 $\mu$m | $d_{13}$ | 160 nm | $n_{13}$ | 24 |
| | | $x_{14}$ | 3.634 $\mu$m | $d_{14}$ | 16 nm | $n_{14}$ | 25 |
| | | $x_{15}$ | 3.953 $\mu$m | $d_{15}$ | 160 nm | $n_{15}$ | 26 |
| | | $x_{16}$ | 4.320 $\mu$m | $d_{16}$ | 160 nm | $n_{16}$ | 28 |
| | | $x_{17}$ | 4.692 $\mu$m | $d_{17}$ | 140 nm | $n_{17}$ | 29 |

**Table S3. GaAs holey antenna design.** ($F_p = 316$, $\eta_2 = 0.87 \rightarrow \eta_{GaAs} = 0.87$)

| Global | | Holes Location | | Holes Diameter | | $N$ | |
|---|---|---|---|---|---|---|---|
| $x_0$ | 5 $\mu$m | $x_1$ | 0.402 $\mu$m | $d_1$ | 77 nm | $n_1$ | 5 |
| $y_0$ | 5 $\mu$m | $x_2$ | 0.557 $\mu$m | $d_2$ | 72 nm | $n_2$ | 6 |
| $H$ | 150 nm | $x_3$ | 0.795 $\mu$m | $d_3$ | 126 nm | $n_3$ | 8 |
| $z_0$ | 1 $\mu$m | $x_4$ | 0.998 $\mu$m | $d_4$ | 135 nm | $n_4$ | 8 |
| $z_{\text{min}}$ | 370 nm | $x_5$ | 1.214 $\mu$m | $d_5$ | 144 nm | $n_5$ | 10 |
| $a_1$ | 1.16 | $x_6$ | 1.452 $\mu$m | $d_6$ | 126 nm | $n_6$ | 12 |
| $a_2$ | 1.08 | $x_7$ | 1.654 $\mu$m | $d_7$ | 90 nm | $n_7$ | 17 |
| theta | 90° | $x_8$ | 1.823 $\mu$m | $d_8$ | 72 nm | $n_8$ | 18 |
| | | $x_9$ | 1.992 $\mu$m | $w_9$ | 72 nm | $n_9$ | 19 |
| | | $x_{10}$ | 2.332 $\mu$m | $d_{10}$ | 63 nm | $n_{10}$ | 20 |
| | | $x_{11}$ | 2.654 $\mu$m | $d_{11}$ | 117 nm | $n_{11}$ | 22 |
| | | $x_{12}$ | 2.965 $\mu$m | $d_{12}$ | 126 nm | $n_{12}$ | 23 |
| | | $x_{13}$ | 3.297 $\mu$m | $d_{13}$ | 144 nm | $n_{13}$ | 24 |
| | | $x_{14}$ | 3.643 $\mu$m | $d_{14}$ | 144 nm | $n_{14}$ | 25 |
| | | $x_{15}$ | 3.963 $\mu$m | $d_{15}$ | 144 nm | $n_{15}$ | 26 |
| | | $x_{16}$ | 4.331 $\mu$m | $d_{16}$ | 144 nm | $n_{16}$ | 28 |
| | | $x_{17}$ | 4.704 $\mu$m | $d_{17}$ | 126 nm | $n_{17}$ | 29 |


2. P. Markos and C. M. Soukoulis, *Wave propagation: from electrons to photonic crystals and left-handed materials* (Princeton University Press, 2008).
3. J. Liu, R. Su, Y. Wei, B. Yao, S. F. C. da Silva, Y. Yu, J. Iles-Smith, K. Srinivasan, A. Rastelli, J. Li *et al.*, "A solid-state source of strongly entangled photon pairs with high brightness and indistinguishability," Nat. Nanotechnol. **14**, 586–593 (2019).
